# Supplementary material for: STEER: Beam Selection for Full-Duplex Millimeter Wave Communication Systems
Source: arXiv:2207.07281 source file (2022-07-15)
Supplement: Supplementary file 1 [file sec-appendix.tex]

\appendices

\section{Test}
